# Supplementary material for: Deep neural network approximation for high-dimensional parabolic partial integro-differential equations
Source: arXiv:2501.10880 source file (2026-10-28)
Supplement: Supplementary file 1 [file final_case.tex]

We are going to take a look at applications for finances.
We refer readers to get familiar with \cite{finacne_intro}.

We take a look at the first simple example.
We assume that our process has jumps always equal to 1 occurring with intensity $\lambda$.
The associated L\'evy measure is $\nu(x) = \lambda\mathds{1}_{\{x=1\}}$ \textcolor{red}{CITATION HERE},
and $\jump$ is always equal to 1, and condition \eqref{D1} has the following form
\begin{equation*}
    \int_{Z} \norm{\jump(t,x,z) - \phif{\jump}(t,x,z)}^2\nu(\dd z)
    =
    \modul{1-\phif{\jump}(t,x,1)}^2
    \leq \delta_c.
\end{equation*}
In the case above it's enough to train DNN always to return 1, and we achieve our desired accuracy.

Another example is a bit more complex.
We consider the following process
\[
    X_t=\sum_{i=1}^{N_t} Y_k - t\lambda\overline{y},
\]
Where $N_t$ is a Poisson process with intensity $\lambda$, and $Y_1,\ Y_2,\dots$ is
identical independent distributed random variables with distributions density function $f$ and
expected value equal to $\overline{y}$.
Then the associated L\'evy measure is $\nu(\dd x) = \lambda f(x)\dd x$ (see~\cite[remark 4.8]{finacne_intro}) and
condition~\eqref{D1} looks as follow
\begin{equation*}
    \lambda\int_{\R}\norm{
        \jump(t,x,z) - \phif{\jump}(t,x,z)
    }^2
    f(x)\dd x \leq \delta_\jump.
\end{equation*}
If we can limit $\norm{
    \jump(t,x,z) - \phif{\jump}(t,x,z)
}$ by $\epsilon$, then
\begin{equation*}
    \lambda\int_{\R}\norm{
        \jump(t,x,z) - \phif{\jump}(t,x,z)
    }^2
    f(x)\dd x\leq \lambda\int_{\R}\epsilon^2
    f(x)\dd x = \lambda \epsilon^2.
\end{equation*}
It was a quick review of how the condition~\eqref{D1} might look in practice.
