# Supplementary material for: Deep neural network approximation for high-dimensional parabolic partial integro-differential equations
Source: arXiv:2501.10880 source file (2026-10-28)
Supplement: Supplementary file 2 [file literature.tex]

\usepackage{amsmath}

As say \cite[Definition 17.4.1]{fayman_kac_Rd} for $a=(a^{ij})$ for $d\times d$ matrix $\sigma\sigma^T$.
Then
\begin{align*}
    \opL_tv(x) &=
    \sum_if^{i}(s,x)\frac{\partial v}{\partial x^i}(x)
    + \frac{1}{2}\sum_{i,j}a^{ij}(s,x)
    \frac{\partial^2 v}{\partial x^i\partial x^j}(x)\\
    &+ \int_{\Z}\at{
        v(x+g(\zeta,s,x))-v(x)
        -\sum_{i}\frac{\partial v}{\partial x^i}g^i(\zeta,s,x)
    }\nu(\zeta).
\end{align*}
We call $\opL$ the infinitesimal generator of the process $X$.
\begin{equation*}
    \dd X_t = f(t,X_t)dt+\sigma(t,X_t)\dd W_t + \int_{\Z}g(\zeta, t, X_{t-})\tilde{\mu}(\dd\zeta, \dd t).
\end{equation*}
This is under assumption where $\mu$ is random measure on $\Z\times[0,\infty]$ with deterministic compensator
$\mu_p(\dd\zeta,\dd t)=\nu(\dd \zeta)\dd t$.
Then $\tilde{\mu} = \mu - \mu_p$.
